# Supplementary material for: Toward a Better Understanding of Probabilistic Delta Debugging
Source: arXiv:2408.04735 source file (2025-05-08)
Supplement: Supplementary file 1 [file appendix.tex]

\section{Appendix}

\subsection{Proofs of important lemmas}
\input{lemmas/lem_same_probability}
\begin{proof}
	If the number of elements in
	\listinput is divisible by the subset size, then each element is placed into
	subsets of equal size. Since the probability update depends entirely on
	the
	current probability and subset size, all elements will have the same
	probability after the update.
\end{proof}

\input{lemmas/lem_increase}
\begin{proof}
	Given $\mysize{r}{} = - \frac{1}{\ln(1 - \myprobability{r}{})}$, we can deduce that $1 - \myprobability{r}{} =
	e^{-\frac{1}{\mysize{r}{}}}$.

	Subsequently, we substitute $1 - \myprobability{r}{}$ into \cref{equation:p_i+1},
	obtaining
	$$\myprobability{r+1}{} = \frac{\myprobability{r}{}}{1 - (1-\myprobability{r}{})^{\mysize{r}{}}} = \frac{\myprobability{r}{}}{1 -
		(e^{-\frac{1}{\mysize{r}{}}})^{\mysize{r}{}}} = \frac{\myprobability{r}{}}{1 - e^{-1}} \approx
	\pincreaseratevalue \times \myprobability{r}{}$$

	Equivalently, the approximate probability
	after round \RoundNumber can be inferred given only \myprobability{0}{}, \ie,
	$$\myprobability{r}{}  = \frac{\myprobability{0}{}}{(1 - e^{-1})^{i}} \approx
	\pincreaseratevalue^{i} \times \myprobability{0}{}$$
\end{proof}

\input{lemmas/lem_relation}
\begin{proof}
	According to \cref{lem:p:increase} and \cref{equation:s_i}, we can
	express
	$\myprobability{r+1}{}$ in terms of $\mysize{r}{}$:
	\begin{align}
		\myprobability{r+1}{} = \frac{\myprobability{r}{}}{1 - e^{-1}} = \frac{1-e^{-\frac{1}{\mysize{r}{}}}}{1 -
			e^{-1}} \label{equation:p_i+1_s_i}
	\end{align}

	Next, we substitute \cref{equation:p_i+1_s_i} into \cref{equation:s_i},
	thus
	representing $\mysize{r+1}{}$ by $\mysize{r}{}$ solely:

	\begin{align}
		\mysize{r+1}{} & = - \frac{1}{\ln(1 - \myprobability{r+1}{})}
		%    = - \frac{1}{\ln(1 - \frac{1 - e^{-\frac{1}{\mysize{r}{}}}}{1 - e^{-1}})}
		%	= -\frac{1}{\ln(\frac{e^{-\frac{1}{\mysize{r}{}}}-e^{-1}}{1 - e^{-1}})}
		%\nonumber \\
		= \frac{1}{\ln(\frac{1 - e^{-1}}{e^{-\frac{1}{\mysize{r}{}}}-e^{-1}})}
		\label{equation:s_complex_final}
	\end{align}
	\label{proof:s_complex_final}
\end{proof}

\begin{lem}
	The lower bound of $\mysize{r+1}{}$ w.r.t $\mysize{r}{}$ is

	\begin{align}
		\mysize{r+1}{} \ge (1 - e^{-1})\mysize{r}{}-1 \label{equation:lowerbound}
	\end{align}
	\label{lem:lower:bound}
\end{lem}
\begin{proof}
	By applying an inequality from Taylor series, \ie, $\forall x \in (0, +\infty),
	ln(x) \le x - 1$, on \cref{lem:s:relation},
	we further transform \cref{equation:s_complex} by removing the
	logarithmic operation
	%\zy{In the following inequality why the fraction becomes its reciprocal?
		%I guess it is a typo?}\mz{fixed}
	\begin{align}
		\mysize{r+1}{} &= \frac{1}{ln(\frac{1 - e^{-1}}{e^{-\frac{1}{\mysize{r}{}}}-e^{-1}})} \ge
		\frac{1}{(\frac{1 - e^{-1}}{e^{-\frac{1}{\mysize{r}{}}}-e^{-1}})-1}
		% 	= \frac{1}{\frac{1 - e^{-\frac{1}{\mysize{r}{}}}}{e^{-\frac{1}{\mysize{r}{}}}-e^{-1}}}
		%\nonumber \\
		%     = \frac{e^{-\frac{1}{\mysize{r}{}}}-e^{-1}}{1 - e^{-\frac{1}{\mysize{r}{}}}}
		= \frac{1-e^{-1}}{1-e^{-\frac{1}{\mysize{r}{}}}}-1 \label{equation:remove_log}
	\end{align}

	Similarly, given that $\forall x \in (-\infty, +\infty), e^{x} \ge x + 1$, we can
	further substitute $e^{-\frac{1}{\mysize{r}{}}}$ in \cref{equation:remove_log}
	with
	$-\frac{1}{\mysize{r}{}} + 1$, obtaining the final linear lower bound:
	\begin{align}
		\mysize{r+1}{} \ge \frac{1-e^{-1}}{1-(-\frac{1}{\mysize{r}{}}+1)}-1 = (1-e^{-1})\mysize{r}{}-1
		\label{equation:lowerbound_final}
	\end{align}
\end{proof}

\begin{lem}
	The upper bound of $\mysize{r+1}{}$ w.r.t $\mysize{r}{}$ is

	\begin{align}
		\mysize{r+1}{} \le (1 - e^{-1})\mysize{r}{} \label{equation:upperbound}
	\end{align}
	\label{lem:upper:bound}
\end{lem}
\begin{proof}
	To prove this inequality always holds,
	we firstly represent $\mysize{r+1}{}$ by $\mysize{r}{}$, thereby
	reformulating $\mysize{r+1}{} \le (1 - e^{-1})\mysize{r}{}$ into
	%$$\mysize{r+1}{} \le (1 - e^{-1})\mysize{r}{}$$
	%$$(1 - e^{-1})\mysize{r}{} \ge \frac{1}{\ln(\frac{1 -
			%e^{-1}}{e^{-\frac{1}{\mysize{r}{}}}-e^{-1}})} $$
	%$$\frac{1}{(1 - e^{-1})\mysize{r}{}} \le \ln(\frac{1 -
		%e^{-1}}{e^{-\frac{1}{\mysize{r}{}}}-e^{-1}})$$

	\begin{align}
		\frac{1}{\ln(\frac{1 - e^{-1}}{e^{-\frac{1}{\mysize{r}{}}}-e^{-1}})} &\le (1 -
		e^{-1})\mysize{r}{}, \mysize{r}{} \in \mathbb{N}, \mysize{r}{} > 1
		\label{equation:reformulate_step2}
	\end{align}

	By assuming $t=-\frac{1}{\mysize{r}{}}$,
	%$$-\frac{t}{(1 - e^{-1})} \le ln(\frac{1 - e^{-1}}{e^{t}-e^{-1}})$$
	%$$\frac{t}{1 - e^{-1}} \ge ln(\frac{e^{t}-e^{-1}}{1 - e^{-1}})$$
	the inequality is transformed to

	\begin{equation}
		f(t) = \frac{t}{1 - e^{-1}} - ln(\frac{e^{t}-e^{-1}}{1 - e^{-1}}) \ge 0, t \in
		(-1,0)
		\label{equation:reformulate}
	\end{equation}

	$f(t)$ decreases monotonically on $(-1, 0)$, because
	$\forall t \in (-1, 0), f'(t) = \frac{1}{1 - e^{-1}} - \frac{1}{1-e^{-1-t}} < 0$.

	Therefore $f(t) \ge f(0) = 0$, indicating that the upper
	bound \cref{equation:upperbound} always holds.
\end{proof}
\begin{figure*}[t]
	\centering
	\includegraphics[width=0.95\linewidth]{figure/bounds.pdf}

	\caption{
		The relationship between the size for next round $\mysize{r+1}{}$ and the
		size for
		current round $\mysize{r}{}$.
		The solid line represents
		$\mysize{r+1}{} = \frac{1}{ln(\frac{1 - e^{-1}}{e^{-\frac{1}{\mysize{r}{}}}-e^{-1}})}$,
		with the dashed lines representing its upper and lower bounds.
%		The enlarged portion represents the curve detail when size is close to 1.
%		The slope slightly changes when size is close to 1, but it does not
%affect the result as the size is always integer and the algorithm terminate
%at
%1.
%        \victor{this image is too large. Make it flatter and shorter}\mz{how about now?}
%        \cn{If you have time, remember to update the font in the pdf file.}
	  }
	\label{fig:bounds}

\end{figure*}

As shown in \cref{fig:bounds}, the original curve does not exceed the
derived upper and lower bounds,
validating our theoretical analysis.

\subsection{Important equations in the paper}
Correlation between subset size and probability.
\begin{empheq}[left=\empheqlbrace]{align}
	\mysize{r}{} &= -\frac{1}{\ln(1 - \myprobability{r}{})}
	\label{equation:s_i} \\
	\myprobability{r+1}{} &= \frac{\myprobability{r}{}}{1 -
		(1-\myprobability{r}{})^{\mysize{r}{}}}
	\label{equation:p_i+1}
\end{empheq}
