# Supplementary material for: Toward a Better Understanding of Probabilistic Delta Debugging
Source: arXiv:2408.04735 source file (2025-05-08)
Supplement: Supplementary file 2 [file icse2025r2-submission-supplementary.pdf]

## APPENDIX

### A. Proofs of important lemmas

**Lemma A.1.** *If the number of elements in  $L$  is always divisible by the subset size, the probabilities of all elements are always the same.*

*Proof.* If the number of elements in  $L$  is divisible by the subset size, then each element is placed into subsets of equal size. Since the probability update depends entirely on the current probability and subset size, all elements will have the same probability after the update.  $\square$

**Lemma A.2.**  *$p$  is increased by a factor  $\frac{1}{1-e^{-1}}$ , i.e.,*

$$p_r = \frac{p_{r-1}}{1-e^{-1}} = \frac{p_0}{(1-e^{-1})^r} \quad (1)$$

*Proof.* Given  $s_r = -\frac{1}{\ln(1-p_r)}$ , we can deduce that  $1-p_r = e^{-\frac{1}{s_r}}$ .

Subsequently, we substitute  $1-p_r$  into Equation (12), obtaining

$$p_{r+1} = \frac{p_r}{1-(1-p_r)^{s_r}} = \frac{p_r}{1-(e^{-\frac{1}{s_r}})^{s_r}} = \frac{p_r}{1-e^{-1}} \approx 1.582 \times p_r$$

Equivalently, the approximate probability after round  $r$  can be inferred given only  $p_0$ , i.e.,

$$p_r = \frac{p_0}{(1-e^{-1})^r} \approx 1.582^r \times p_0$$

**Lemma A.3.**  *$s_{r+1}$  can be expressed by solely  $s_r$*

$$s_{r+1} = \frac{1}{\ln\left(\frac{1-e^{-1}}{e^{-\frac{1}{s_r}}-e^{-1}}\right)} \quad (2)$$

*Proof.* According to Theorem A.2 and Equation (11), we can express  $p_{r+1}$  in terms of  $s_r$ :

$$p_{r+1} = \frac{p_r}{1-e^{-1}} = \frac{1-e^{-\frac{1}{s_r}}}{1-e^{-1}} \quad (3)$$

Next, we substitute Equation (3) into Equation (11), thus representing  $s_{r+1}$  by  $s_r$  solely:

$$s_{r+1} = -\frac{1}{\ln(1-p_{r+1})} = \frac{1}{\ln\left(\frac{1-e^{-1}}{e^{-\frac{1}{s_r}}-e^{-1}}\right)} \quad (4)$$

$\square$

**Lemma A.4.** *The lower bound of  $s_{r+1}$  w.r.t  $s_r$  is*

$$s_{r+1} \geq (1-e^{-1})s_r - 1 \quad (5)$$

*Proof.* By applying an inequality from Taylor series, i.e.,  $\forall x \in (0, +\infty), \ln(x) \leq x-1$ , on Theorem A.3, we further transform Equation (2) by removing the logarithmic operation

$$s_{r+1} = \frac{1}{\ln\left(\frac{1-e^{-1}}{e^{-\frac{1}{s_r}}-e^{-1}}\right)} \geq \frac{1}{\left(\frac{1-e^{-1}}{e^{-\frac{1}{s_r}}-e^{-1}}\right)-1} = \frac{1-e^{-1}}{1-e^{-\frac{1}{s_r}}} - 1 \quad (6)$$

Similarly, given that  $\forall x \in (-\infty, +\infty), e^x \geq x+1$ , we can further substitute  $e^{-\frac{1}{s_r}}$  in Equation (6) with  $-\frac{1}{s_r}+1$ , obtaining the final linear lower bound:

$$s_{r+1} \geq \frac{1-e^{-1}}{1-\left(-\frac{1}{s_r}+1\right)} - 1 = (1-e^{-1})s_r - 1 \quad (7)$$

$\square$

**Lemma A.5.** *The upper bound of  $s_{r+1}$  w.r.t  $s_r$  is*

$$s_{r+1} \leq (1-e^{-1})s_r \quad (8)$$

*Proof.* To prove this inequality always holds, we firstly represent  $s_{r+1}$  by  $s_r$ , thereby reformulating  $s_{r+1} \leq (1-e^{-1})s_r$  into

$$\frac{1}{\ln\left(\frac{1-e^{-1}}{e^{-\frac{1}{s_r}}-e^{-1}}\right)} \leq (1-e^{-1})s_r, s_r \in \mathbb{N}, s_r > 1 \quad (9)$$

By assuming  $t = -\frac{1}{s_r}$ , the inequality is transformed to

$$f(t) = \frac{t}{1-e^{-1}} - \ln\left(\frac{e^t - e^{-1}}{1-e^{-1}}\right) \geq 0, t \in (-1, 0) \quad (10)$$

$\square$

$f(t)$  decreases monotonically on  $(-1, 0)$ , because  $\forall t \in (-1, 0), f'(t) = \frac{1}{1-e^{-1}} - \frac{1}{1-e^{-1-t}} < 0$ .

Therefore  $f(t) \geq f(0) = 0$ , indicating that the upper bound Equation (8) always holds.  $\square$

As shown in Fig. 1, the original curve does not exceed the derived upper and lower bounds, validating our theoretical analysis.

### B. Important equations in the paper

Correlation between subset size and probability.

$$\begin{cases} s_r = -\frac{1}{\ln(1-p_r)} \end{cases} \quad (11)$$

$$\begin{cases} p_{r+1} = \frac{p_r}{1-(1-p_r)^{s_r}} \end{cases} \quad (12)$$

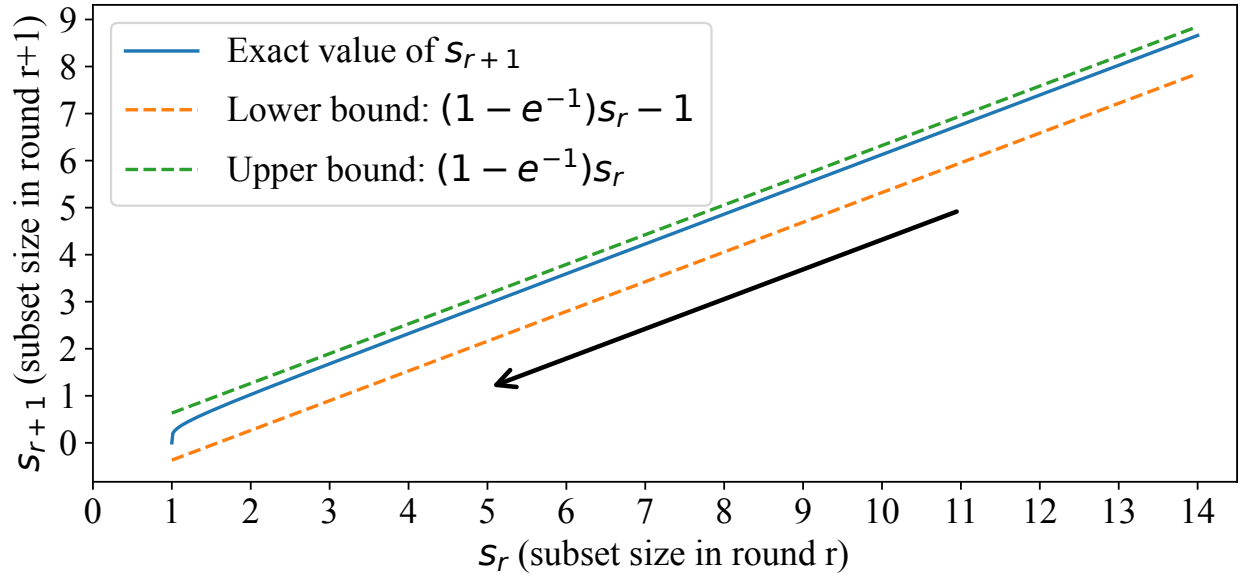

Fig. 1: The relationship between the size for next round  $s_{r+1}$  and the size for current round  $s_r$ . The solid line represents  $s_{r+1} = \frac{1}{\ln(\frac{1-e^{-1}}{-\frac{1}{e^{s_r}} - e^{-1}})}$ , with the dashed lines representing its upper and lower bounds.
